# Supplementary material for: Geometry and dynamics of lipid membranes: The Scriven--Love number
Source: arXiv:1910.10693 source file (2020-05-05)
Supplement: Supplementary file 1 [file appendix.tex]

\section{Tube Pulling Force}

We calculate now.
